# Supplementary material for: Covariate-guided Bayesian mixture model for multivariate time series
Source: arXiv:2301.01373 source file (2023-01-03)
Supplement: Supplementary file 1 [file supplemental_v3_0930.pdf]

# Supplemental materials for “Covariate-Guided Bayesian Mixture of Spline Experts for the Analysis of Multivariate Time Series”

Haoyi Fu, Lu Tang, Ori Rosen, Alison E. Hipwell,

Theodore J. Huppert, Robert T. Krafty

September 30, 2022

## APPENDIX A: DETAILS OF THE SAMPLING SCHEME

As described in the Section 5 of the paper, Gibbs sampling is used as the sampling scheme. We denote  $\boldsymbol{\Theta}_{gk} = (\boldsymbol{\theta}'_{gk}, \tau_{gk}^2, \sigma_{gk}^2, \boldsymbol{\delta}_g^{*'}, \kappa_g^2)'$  as parameters for  $g$ th component and  $k$ th entry. Model parameters (linear, basis function coefficients, error variances and smoothing parameters) for each component and entry are drawn from their conditional posterior distributions, while other parameters (logistic parameters, random intercepts and variance of random intercepts) for each component are drawn from their conditional posterior distributions. Detailed Gibbs sampling scheme is given as below.

### 1. Sampling basis function coefficients

For each component  $g$  and time series entry  $k$ , based on the augmented likelihood in Section 3.3 and priors on  $\boldsymbol{\theta}_{gk} = (\boldsymbol{\alpha}'_{gk}, \boldsymbol{\beta}'_{gk})'$  in Section 4.1, the conditional posterior distribution of  $\boldsymbol{\theta}_{gk} | \mathbf{y}, \mathbf{S}, \tau_{gk}^2, \sigma_{gk}^2$  is:

$$\begin{aligned}
p(\boldsymbol{\theta}_{gk} | \mathbf{y}, \mathbf{S}, \tau_{gk}^2, \sigma_{gk}^2) &\propto p(\mathbf{y} | \mathbf{S}, \boldsymbol{\theta}_{gk}, \sigma_{gk}^2) p(\boldsymbol{\theta}_{gk} | \tau_{gk}^2) \\
&\propto \prod_{i=1}^N [(\sigma_{gk}^2)^{-n/2} \exp\{-\frac{1}{2\sigma_{gk}^2} (\mathbf{y}_{ik} - \mathbf{S}\boldsymbol{\theta}_{gk})' (\mathbf{y}_{ik} - \mathbf{S}\boldsymbol{\theta}_{gk})\}]^{z_{ig}} \\
&\times |\mathbf{D}_{gk}|^{-1/2} \exp\{-\frac{1}{2} \boldsymbol{\theta}_{gk}' \mathbf{D}_{gk}^{-1} \boldsymbol{\theta}_{gk}\} \\
&\propto \exp\{-\frac{1}{2\sigma_{gk}^2} [\sum_{i=1}^N z_{ig} (\mathbf{y}_{ik} - \mathbf{S}\boldsymbol{\theta}_{gk})' (\mathbf{y}_{ik} - \mathbf{S}\boldsymbol{\theta}_{gk}) + \boldsymbol{\theta}_{gk}' \sigma_{gk}^2 \mathbf{D}_{gk}^{-1} \boldsymbol{\theta}_{gk}]\} \\
&\propto \exp\{-\frac{1}{2\sigma_{gk}^2} (\boldsymbol{\theta}_{gk} - \mathbf{u}_{gk})' (\boldsymbol{\Lambda}_{gk})^{-1} (\boldsymbol{\theta}_{gk} - \mathbf{u}_{gk})\} \\
&\sim N(\mathbf{u}_{gk}, \sigma_{gk}^2 \boldsymbol{\Lambda}_{gk}),
\end{aligned}$$

where  $\boldsymbol{\Lambda}_{gk} = (N_g \mathbf{S}' \mathbf{S} + \sigma_{gk}^2 \mathbf{D}_{gk}^{-1})^{-1}$  and  $\mathbf{u}_{gk} = \boldsymbol{\Lambda}_{gk} \sum_{i=1}^N z_{ig} \mathbf{S}' \mathbf{y}_{ik}$ ,  $N_g$  is the number of multivariate time series that belongs to the  $g$ th component,  $\mathbf{D}_{gk} = \text{diag}(\sigma_{gk}^2 \mathbf{1}_2, \tau_{gk}^2 \mathbf{1}_m)$  is the prior covariance matrix for  $\boldsymbol{\theta}_{gk}$ . Hence, for each component  $g$  and entry  $k$ , we can draw  $\boldsymbol{\theta}_{gk} | \sigma_{gk}^2, \tau_{gk}^2, \mathbf{y}, \mathbf{S} \sim N(\mathbf{u}_{gk}, \sigma_{gk}^2 \boldsymbol{\Lambda}_{gk})$ .

## 2. Sampling error variances

Gelman (2006) used the half-t distribution as prior distribution of scale parameters. We follow Wand *and others* (2011) and expand the half-t prior in Section 4.3 by augmenting the posterior of error variances with a latent variable  $a_{\sigma_{gk}}$  and the following hierarchical structure

$$\sigma_{gk}^2 | a_{\sigma_{gk}} \sim IG(\frac{\nu_\sigma}{2}, \frac{\nu_\sigma}{a_{\sigma_{gk}}}), a_{\sigma_{gk}} \sim IG(\frac{1}{2}, \frac{1}{A_\sigma^2}).$$

Therefore, the conditional posterior distribution of the latent variable is

$$p(a_{\sigma_{gk}} | \sigma_{gk}^2) \propto p(\sigma_{gk}^2 | a_{\sigma_{gk}}) p(a_{\sigma_{gk}}) \propto \exp\left(-\frac{1}{a_{\sigma_{gk}}} \left(\frac{\nu_\sigma}{\sigma_{gk}^2} + \frac{1}{A_\sigma^2}\right)\right) (a_{\sigma_{gk}})^{-(\frac{1}{2}+1+\frac{\nu_\sigma}{2})},$$

which can be sampled from  $IG(\frac{\nu_\sigma+1}{2}, \frac{\nu_\sigma}{\sigma_{gk}^2} + \frac{1}{A_\sigma^2})$ . Denoting  $\boldsymbol{\epsilon}_{igk}$  as the error vector of the time series  $\mathbf{y}_{ik}$  for the component  $g$  and we have  $\boldsymbol{\epsilon}_{igk} = \mathbf{y}_{ik} - \mathbf{S}\boldsymbol{\theta}_{gk}$ , where  $\boldsymbol{\epsilon}_{igk} \sim N(\mathbf{0}, \sigma_{gk}^2 \mathbf{I}_n)$ .

The conditional distribution of the error variance is

$$\begin{aligned}
p(\sigma_{gk}^2 | \epsilon_{igk}, a_{\sigma_{gk}}) &\propto p(\epsilon_{igk} | \sigma_{gk}^2) p(a_{\sigma_{gk}} | \sigma_{gk}^2) p(\sigma_{gk}^2) \\
&\propto \prod_{i=1}^N [(\sigma_{gk}^2)^{-\frac{n}{2}} \exp(-\frac{1}{2\sigma_{gk}^2} \epsilon'_{igk} \epsilon_{igk})]^{z_{ig}} \times (\sigma_{gk}^2)^{-(\frac{\nu_\sigma}{2}+1)} \exp(-\frac{\nu_\sigma}{\sigma_{gk}^2 a_{\sigma_{gk}}}) \\
&\propto (\sigma_{gk}^2)^{-(\frac{n}{2}N_g + \frac{\nu_\sigma}{2}+1)} \exp\left(-\frac{1}{\sigma_{gk}^2} \left(\frac{\sum_{i=1}^N z_{ig} \epsilon'_{igk} \epsilon_{igk}}{2} + \frac{\nu_\sigma}{a_{\sigma_{gk}}}\right)\right),
\end{aligned}$$

which can be sampled from  $IG(\frac{nN_g + \nu_\sigma}{2}, \frac{\sum_{i=1}^N z_{ig} \epsilon'_{igk} \epsilon_{igk}}{2} + \frac{\nu_\sigma}{a_{\sigma_{gk}}})$ . The sampling scheme proceeds by first sampling  $a_{\sigma_{gk}} | \sigma_{gk}^2$  than  $\sigma_{gk}^2 | \epsilon_{igk}, a_{\sigma_{gk}}$ .

### 3. Sampling smoothing parameters

Following the same procedure as sampling error variances, we can sample the smoothing parameter  $\tau_{gk}^2$  by introducing a latent variable  $a_{\tau_{gk}}$ . We first draw  $a_{\tau_{gk}} | \tau_{gk}^2 \sim IG(\frac{\nu_\tau + 1}{2}, \frac{\nu_\tau}{\tau_{gk}^2} + \frac{1}{A_\tau^2})$  and the conditional posterior distribution of the smoothing parameter is

$$\begin{aligned}
p(\tau_{gk}^2 | \beta_{gk}, a_{\tau_{gk}}) &\propto p(\beta_{gk} | \tau_{gk}^2) p(a_{\tau_{gk}} | \tau_{gk}^2) p(\tau_{gk}^2) \\
&\propto (\tau_{gk}^2)^{-\frac{m + \nu_\tau}{2}} \exp\left(-\frac{1}{\tau_{gk}^2} \left(\frac{\nu_\tau}{a_{\tau_{gk}}} + \frac{\beta'_{gk} \beta_{gk}}{2}\right)\right),
\end{aligned}$$

which can be sampled from  $IG(\frac{\nu_\tau + m}{2}, \frac{\beta'_{gk} \beta_{gk}}{2} + \frac{\nu_\tau}{a_{\tau_{gk}}})$ . The sampling scheme proceeds by first sampling  $a_{\tau_{gk}} | \tau_{gk}^2$  then  $\tau_{gk}^2 | \beta_{gk}, a_{\tau_{gk}}$ .

### 4. Sampling logistic parameters

Based on the model for mixing weights in Section 3.2 and priors of logistic parameters in Section 4.4, the conditional posterior distributions of  $\delta_g^* | z_{ig}, \kappa_g^2, \mathbf{V}^*$  are

$$\begin{aligned}
p(\delta_g^* | z_{ig}, \kappa_g^2, \mathbf{V}^*) &\propto p(z_{ig} = 1 | \delta_g^*, \mathbf{V}^*) p(\delta_g^* | \kappa_g^2) \\
&= \prod_{i=1}^N \left( \frac{\exp(\mathbf{V}_i^{*'} \delta_g^*)}{\sum_{h=1}^G \exp(\mathbf{V}_i^{*'} \delta_h^*)} \right)^{z_{ig}} p(\delta_g^* | \kappa_g^2),
\end{aligned}$$

where  $\mathbf{V}^* = (\mathbf{V}_1^*, \dots, \mathbf{V}_N^*)'$  is a  $N \times (P+1)$  matrix with  $\mathbf{V}_i^*$  representing all covariates (including intercepts) for subject  $i$ . To sample from the posterior distribution of  $p(\delta_g^* | z_{ig}, \kappa_g^2, \mathbf{V}^*)$ , we

adopt the Pólya-Gamma data augmentation strategy from Polson *and others* (2013) by introducing a latent Pólya-Gamma variable  $\omega_{ig}$ , which comes from the Pólya-Gamma distribution. Thus, the conditional posterior distributions of the logistic parameters are

$$\begin{aligned} p(\boldsymbol{\delta}_g^* | z_{ig}, \omega_{ig}, \kappa_g^2, \mathbf{V}^*) &\propto p(z_{ig} = 1 | \omega_{ig}, \boldsymbol{\delta}_g^*, \mathbf{V}^*) p(\boldsymbol{\delta}_g^* | \kappa_g^2) \\ &\propto \exp\left(-\frac{\omega_{ig} \eta_{ig}^2}{2}\right) p(\omega_{ig} | 1, 0) |\mathbf{B}_g|^{-P/2} \exp\left\{-\frac{1}{2} \boldsymbol{\delta}_g^{*'} \mathbf{B}_g^{-1} \boldsymbol{\delta}_g^*\right\}, \end{aligned}$$

where  $\eta_{ig} = \mathbf{V}_i^{*'} \boldsymbol{\delta}_g^* - C_{ig}$  and  $C_{ig} = \log \sum_{h \neq j} \exp(\mathbf{V}_i^{*'} \boldsymbol{\delta}_h^*)$ ,  $p(\omega_{ig} | 1, 0)$  is the Pólya-gamma distribution  $PG(b, c)$  with  $b = 1$  and  $c = 0$ ,  $\mathbf{B}_g$  is the prior covariance matrix from Section 4.4 and  $\mathbf{B}_g = \text{diag}(\sigma_B^2 \mathbf{I}_{P+1}, \kappa_g^2 \mathbf{I}_N)$ . By assuming the conjugate prior for  $\boldsymbol{\delta}_g^*$ , which follows  $N(\mathbf{0}, \mathbf{B}_g)$ . The posterior distribution of the Pólya-gamma latent variable is

$$\omega_{ig} | \boldsymbol{\delta}_g^*, \mathbf{V}^* \sim PG(1, \eta_{ig}).$$

Thus, the conditional distributions of logistic parameters (including random intercepts) are

$$\boldsymbol{\delta}_g^* | z_{ig}, \omega_{ig}, \kappa_g^2, \mathbf{V}^* \sim N(\mathbf{M}_g, \boldsymbol{\Sigma}_g),$$

where posterior variance  $\boldsymbol{\Sigma}_g = (\mathbf{V}^{*'} \boldsymbol{\Omega}_g \mathbf{V}^* + \mathbf{B}_g^{-1})^{-1}$  and posterior mean  $\mathbf{M}_g = \boldsymbol{\Sigma}_g (\mathbf{V}^{*'} (\boldsymbol{\Omega}_g \mathbf{C}_g + \boldsymbol{\xi}_g))$ . We have  $\boldsymbol{\Omega}_g = \text{diag}(\omega_{1g}, \dots, \omega_{Ng})$ ,  $\mathbf{C}_g = (C_{1g}, \dots, C_{Ng})'$ , and  $\boldsymbol{\xi}_g = (\xi_{1g}, \dots, \xi_{Ng})'$ , where  $\xi_{ig} = z_{ig} - \frac{1}{2}$ . Thus,  $\boldsymbol{\delta}_g^*$  can be drawn by first sampling  $\omega_{ig} | \boldsymbol{\delta}_g^*, \mathbf{V}^*$  and then sampling  $\boldsymbol{\delta}_g^* | z_{ig}, \omega_{ig}, \kappa_g^2, \mathbf{V}^*$ .

## 5. Sampling variances of random intercepts

Following the same procedure as sampling error variances and smoothing parameters, we first draw  $a_{\kappa_g} | \kappa_g^2 \sim IG(\frac{\nu_\kappa + 1}{2}, \frac{\nu_\kappa}{\kappa_g^2} + \frac{1}{A_\kappa^2})$  and the conditional posterior distribution of the variance of random intercepts is

$$\begin{aligned} p(\kappa_g^2 | \boldsymbol{\zeta}_g, a_{\kappa_g}) &\propto p(\boldsymbol{\zeta}_g | \kappa_g^2) p(a_{\kappa_g} | \kappa_g^2) p(\kappa_g^2) \\ &\propto (\kappa_g^2)^{-\frac{N + \nu_\kappa}{2} + 1} \exp\left(-\frac{1}{\kappa_g^2} \left(\frac{\nu_\kappa}{a_{\kappa_g}} + \frac{\boldsymbol{\zeta}_g^T \boldsymbol{\zeta}_g}{2}\right)\right), \end{aligned}$$

which can be sampled from  $IG(\frac{\nu_{\kappa}+N}{2}, \frac{\zeta_g^T \zeta_g}{2} + \frac{\nu_{\kappa}}{a_{\kappa_g}})$ . The sampling scheme proceeds by first sampling  $a_{\kappa_g} | \kappa_g^2$  than  $\kappa_g^2 | \zeta_g, a_{\kappa_g}$ .

## 6. Computing mixing weights

After drawing  $\delta_g^*$  from the posterior distributions, we can directly compute mixing weights  $\pi_{ig}$  for each component with known design matrix  $V^*$  by

$$\pi_{ig}(V_i^*) = \frac{\exp(V_i^{*T} \delta_g^*)}{\sum_{h=1}^G \exp(V_i^{*T} \delta_h^*)},$$

where we denote  $\delta_g^* = (\delta_g^T, \zeta_g^T)^T$  as the aggregation of logistic parameters and all random intercepts for the  $g$ th component.

## 7. Sampling latent indicators

After obtaining all parameters and mixing weights, the final step is to allocate subjects to different components by sampling the latent indicator  $z_{ig}$ . The latent indicator  $z_{ig}$  has the following distribution as in Section 3.3:

$$f(z_{ig} = 1 | \Theta_g, \mathbf{S}, \mathbf{y}_i) = \frac{\pi_{ig} \prod_{j=1}^n f_g(\mathbf{y}_{it_j} | \Theta_g)}{\sum_{h=1}^G \pi_{ih} \prod_{j=1}^n f_h(\mathbf{y}_{it_j} | \Theta_h)},$$

which can be drawn directly from the multinomial distribution.

## APPENDIX B: ADDITIONAL SIMULATION RESULTS

Appendix B adds more simulation results in addition to simulation results in the paper. To further demonstrate the performance of the proposed method, we conduct simulation studies based on two scenarios: the two-component trivariate regression spline and the four-component bivariate regression spline model. The model formula is displayed in Section 6.1 of the paper. We investigate the performance of our proposed method in terms of estimated trajectories and logistic parameters

Mean(SD) of the ARSE, A-bias and V-bias of estimated trajectories of the two-component trivariate model are given in Table S1. To demonstrate the performance of the proposed method in various settings, we look at combinations of the number of multivariate time series ( $N = 150, 250$ ) and the length of each univariate time series ( $n = 50, 70$ ), and compare our proposed method to

two existing methods: *gbmt* package in R (Magrini, 2022) and *TRAJ* procedure in SAS (Nagin and others, 2018). The case of  $n = 50$  and  $N = 150$  in Table S1 corresponds to the Figure 3 in the paper. The performance of logistic parameters (RMSEs) with different  $n$  and  $N$  are given in Table 1 of the paper.

Mean(SD) of the ARSE, A-bias and V-bias of estimated trajectories of  $N = 150$  four-component bivariate time series of length  $n = 50$  are given in Table S2, which correspond to Figure 4 in the paper. RMSEs of logistic parameters for this setting are listed in Table 2 of the paper. Tables S3 - S8 give the performance of estimated trajectories and logistic parameters for combinations of different lengths of time series  $n$  and numbers of time series  $N$ , under the scenario of the four-component bivariate model.

As expected, our proposed method outperforms the two existing methods in terms of estimated trajectories for each component under different settings (different  $n$  and  $N$ , both two-component trivariate and four-component bivariate scenarios). The proposed method is able to achieve a smaller ARSE and V-bias, while all three methods are able to obtain estimated trajectories with a very small bias. Notably, for the four-component bivariate scenario, *TRAJ* gives larger values of mean ARSE, A-bias and V-bias, which result from imprecise estimates of several replicates due to the convergence issue. In terms of logistic parameters, our proposed method outperforms *TRAJ* in almost all comparisons, especially for the intercept  $\delta_0$  and the first covariate  $\delta_1$ . Our proposed method is able to give shrinkage estimates of logistic parameters with the use of the Bayesian method, while multinomial logistic regression used in the *TRAJ* would give inflated parameter estimates in cases of perfect separations and unbalanced designs.

Table S1: Mean (standard deviation) of the averaged root square error (ARSE), the averaged bias (A-bias) and the variance of bias (V-bias) of estimated trajectories for each component from 100 replicates of  $N$  two-component trivariate time series of length  $n$ . Estimates of the proposed method were compared to R package gbmt and TRAJ procedure in SAS. C1 and C2 denote first and second components. Means were calculated by averaging over estimates of 100 replicates. Standard deviations are Monte Carlo standard deviations from estimates of 100 replicates. Each value was reported  $\times 10^2$ .

| n  | N   | Method   | ARSE C1 | A-bias C1 | V-bias C1 | ARSE C2 | A-bias C2 | V-bias C2 |
|----|-----|----------|---------|-----------|-----------|---------|-----------|-----------|
| 50 | 150 | Proposed | 8.35    | 0.03      | 0.68      | 7.65    | 0.10      | 0.58      |
|    |     |          | (1.26)  | (1.83)    | (0.22)    | (1.38)  | (1.76)    | (0.22)    |
|    |     | gbmt     | 10.67   | 0.03      | 1.15      | 9.08    | 0.10      | 0.83      |
|    |     |          | (1.91)  | (1.83)    | (0.42)    | (1.72)  | (1.76)    | (0.33)    |
|    |     | TRAJ     | 11.06   | 0.03      | 1.22      | 10.59   | 0.10      | 1.12      |
|    |     |          | (1.48)  | (1.83)    | (0.33)    | (1.52)  | (1.76)    | (0.34)    |
| 70 | 150 | Proposed | 7.16    | 0.24      | 0.51      | 6.53    | -0.11     | 0.42      |
|    |     |          | (1.04)  | (1.38)    | (0.16)    | (1.07)  | (1.42)    | (0.14)    |
|    |     | gbmt     | 9.91    | 0.24      | 1.01      | 8.19    | -0.11     | 0.68      |
|    |     |          | (1.96)  | (1.38)    | (0.40)    | (1.65)  | (1.42)    | (0.29)    |
|    |     | TRAJ     | 9.34    | 0.24      | 0.87      | 8.95    | -0.11     | 0.80      |
|    |     |          | (1.10)  | (1.38)    | (0.22)    | (1.13)  | (1.42)    | (0.20)    |
| 50 | 250 | Proposed | 6.81    | 0.07      | 0.46      | 6.22    | 0.02      | 0.38      |
|    |     |          | (1.02)  | (1.33)    | (0.14)    | (0.94)  | (1.31)    | (0.12)    |
|    |     | gbmt     | 9.79    | 0.07      | 0.98      | 8.00    | 0.02      | 0.65      |
|    |     |          | (1.91)  | (1.33)    | (0.40)    | (1.53)  | (1.31)    | (0.26)    |
|    |     | TRAJ     | 8.70    | 0.07      | 0.76      | 8.20    | 0.02      | 0.67      |
|    |     |          | (1.18)  | (1.33)    | (0.21)    | (1.03)  | (1.31)    | (0.17)    |
| 70 | 250 | Proposed | 5.65    | 0.08      | 0.32      | 5.27    | -0.06     | 0.27      |
|    |     |          | (0.84)  | (1.00)    | (0.10)    | (0.82)  | (1.42)    | (0.09)    |
|    |     | gbmt     | 9.15    | 0.08      | 0.87      | 7.43    | -0.06     | 0.56      |
|    |     |          | (1.96)  | (1.00)    | (0.38)    | (1.60)  | (1.42)    | (0.26)    |
|    |     | TRAJ     | 7.18    | 0.08      | 0.52      | 6.80    | -0.06     | 0.45      |
|    |     |          | (0.94)  | (1.00)    | (0.14)    | (0.77)  | (1.42)    | (0.10)    |

Table S2: Mean (standard deviation) of the averaged root square error (ARSE), the averaged bias (A-bias) and the variance of bias (V-bias) of estimated trajectories for each component from 100 replicates of 150 four-component bivariate time series of length 50. Estimates of the proposed method were compared to R package gbmt and TRAJ procedure in SAS. C1, C2, C3 and C4 denote first, second, third and fourth component, respectively. Means were calculated by averaging over estimates of 100 replicates. Standard deviations are Monte Carlo standard deviations from estimates of 100 replicates. Each value was reported  $\times 10^2$ .

| n  | N   | Method   | ARSE C1 | A-bias C1 | V-bias C1 | ARSE C2 | A-bias C2 | V-bias C2 |
|----|-----|----------|---------|-----------|-----------|---------|-----------|-----------|
| 50 | 150 | Proposed | 4.38    | 0.38      | 0.18      | 3.76    | -0.01     | 0.13      |
|    |     |          | (1.04)  | (1.59)    | (0.08)    | (0.87)  | (1.37)    | (0.06)    |
|    |     | gbmt     | 4.75    | 0.38      | 0.21      | 4.79    | 0.01      | 0.22      |
|    |     |          | (1.04)  | (1.59)    | (0.09)    | (1.17)  | (1.65)    | (0.11)    |
|    |     | TRAJ     | 13.87   | 0.62      | 3.39      | 12.41   | 0.08      | 2.41      |
|    |     |          | (15.59) | (9.91)    | (9.24)    | (13.42) | (9.74)    | (5.37)    |
| n  | N   | Method   | ARSE C3 | A-bias C3 | V-bias C3 | ARSE C4 | A-bias C4 | V-bias C4 |
| 50 | 150 | Proposed | 4.69    | -0.11     | 0.20      | 3.88    | -0.09     | 0.14      |
|    |     |          | (1.14)  | (1.83)    | (0.12)    | (1.15)  | (1.56)    | (0.08)    |
|    |     | gbmt     | 5.08    | -0.12     | 0.24      | 4.70    | -0.09     | 0.21      |
|    |     |          | (1.12)  | (1.83)    | (0.12)    | (1.32)  | (1.78)    | (0.12)    |
|    |     | TRAJ     | 14.55   | -1.58     | 3.24      | 14.36   | 0.12      | 3.99      |
|    |     |          | (14.82) | (10.31)   | (7.35)    | (17.01) | (9.92)    | (10.70)   |

Table S3: Mean (standard deviation) of the averaged root square error (ARSE), the averaged bias (A-bias) and the variance of bias (V-bias) of estimated trajectories for each component from 100 replicates of 150 four-component bivariate time series of length 70. Estimates of the proposed method were compared to R package gbmt and TRAJ procedure in SAS. C1, C2, C3 and C4 denote first, second, third and fourth component, respectively. Means were calculated by averaging over estimates of 100 replicates. Standard deviations are Monte Carlo standard deviations from estimates of 100 replicates. Each value was reported  $\times 10^2$ .

| n  | N   | Method   | ARSE C1 | A-bias C1 | V-bias C1 | ARSE C2 | A-bias C2 | V-bias C2 |
|----|-----|----------|---------|-----------|-----------|---------|-----------|-----------|
| 70 | 150 | Proposed | 3.82    | 0.44      | 0.14      | 3.22    | -0.07     | 0.10      |
|    |     |          | (0.95)  | (1.30)    | (0.07)    | (0.85)  | (0.95)    | (0.06)    |
|    |     | gbmt     | 4.05    | 0.44      | 0.16      | 4.11    | -0.08     | 0.17      |
|    |     |          | (0.97)  | (1.30)    | (0.08)    | (1.12)  | (1.15)    | (0.10)    |
|    |     | TRAJ     | 13.51   | -0.30     | 3.86      | 10.00   | -0.25     | 1.64      |
|    |     |          | (17.04) | (9.34)    | (10.73)   | (10.11) | (6.21)    | (4.02)    |
| n  | N   | Method   | ARSE C3 | A-bias C3 | V-bias C3 | ARSE C4 | A-bias C4 | V-bias C4 |
| 70 | 150 | Proposed | 4.12    | -0.29     | 0.15      | 3.52    | 0.24      | 0.12      |
|    |     |          | (0.90)  | (1.69)    | (0.06)    | (0.85)  | (1.22)    | (0.06)    |
|    |     | gbmt     | 4.38    | -0.29     | 0.17      | 4.13    | 0.27      | 0.16      |
|    |     |          | (1.01)  | (1.69)    | (0.07)    | (0.99)  | (1.40)    | (0.09)    |
|    |     | TRAJ     | 13.03   | 0.30      | 3.86      | 11.77   | 0.39      | 2.57      |
|    |     |          | (17.04) | (10.49)   | (10.73)   | (13.78) | (8.49)    | (6.45)    |



Table S4: Root mean square errors (RMSEs) of each logistic parameter for the four-component bivariate model from 100 replicates of 150 four-component bivariate time series of length 70. RMSEs of the proposed method were compared to TRAJ procedure in SAS. Parameters  $\delta_0$ ,  $\delta_1$ ,  $\delta_2$  and  $\delta_3$  are intercept, first, second and third logistic parameters, respectively. The fourth component was used as the reference component. The true values of logistic parameters are 5,  $-3.5$ , 1, 0.1 (first component),  $-4$ , 2.5,  $-2$ ,  $-0.2$  (second component), 3,  $-2$ , 0.8, 0.2 (third component). C1, C2, C3 and C4 denote first, second, third and fourth component, respectively.

| n  | N   | Method   | Comparison | $\delta_0$ | $\delta_1$ | $\delta_2$ | $\delta_3$ |
|----|-----|----------|------------|------------|------------|------------|------------|
| 70 | 150 | Proposed | C1 vs C4   | 0.81       | 0.51       | 0.29       | 0.41       |
|    |     |          | C2 vs C4   | 1.42       | 0.73       | 0.58       | 0.36       |
|    |     |          | C3 vs C4   | 1.05       | 0.58       | 0.37       | 0.31       |
|    |     | TRAJ     | C1 vs C4   | 1.13       | 0.66       | 0.31       | 0.45       |
|    |     |          | C2 vs C4   | 3.12       | 1.66       | 0.99       | 0.55       |
|    |     |          | C3 vs C4   | 1.15       | 0.74       | 0.48       | 0.35       |

Table S5: Mean (standard deviation) of the averaged root square error (ARSE), the averaged bias (A-bias) and the variance of bias (V-bias) of estimated trajectories for each component from 100 replicates of 250 four-component bivariate time series of length 50. Estimates of the proposed method were compared to R package gbmt and TRAJ procedure in SAS. C1, C2, C3 and C4 denote first, second, third and fourth component, respectively. Means were calculated by averaging over estimates of 100 replicates. Standard deviations are Monte Carlo standard deviations from estimates of 100 replicates. Each value was reported  $\times 10^2$ .

| n  | N   | Method   | ARSE C1 | A-bias C1 | V-bias C1 | ARSE C2 | A-bias C2 | V-bias C2 |
|----|-----|----------|---------|-----------|-----------|---------|-----------|-----------|
| 50 | 250 | Proposed | 3.42    | 0.18      | 0.11      | 2.86    | -0.14     | 0.08      |
|    |     |          | (0.78)  | (1.19)    | (0.05)    | (0.61)  | (0.98)    | (0.04)    |
|    |     | gbmt     | 3.57    | 0.18      | 0.12      | 3.68    | -0.15     | 0.13      |
|    |     |          | (0.85)  | (1.19)    | (0.06)    | (0.79)  | (1.20)    | (0.06)    |
|    |     | TRAJ     | 11.66   | 0.53      | 2.50      | 8.90    | 1.47      | 1.05      |
|    |     |          | (15.03) | (10.63)   | (6.30)    | (9.38)  | (7.81)    | (2.16)    |
| n  | N   | Method   | ARSE C3 | A-bias C3 | V-bias C3 | ARSE C4 | A-bias C4 | V-bias C4 |
| 50 | 250 | Proposed | 3.93    | -0.06     | 0.14      | 3.28    | -0.10     | 0.10      |
|    |     |          | (0.92)  | (1.48)    | (0.07)    | (0.76)  | (1.19)    | (0.05)    |
|    |     | gbmt     | 4.16    | -0.06     | 0.16      | 3.83    | -0.13     | 0.14      |
|    |     |          | (0.95)  | (1.49)    | (0.07)    | (0.83)  | (1.36)    | (0.06)    |
|    |     | TRAJ     | 10.80   | 0.49      | 1.83      | 10.17   | -0.17     | 1.84      |
|    |     |          | (9.92)  | (5.78)    | (3.70)    | (12.54) | (8.83)    | (5.20)    |

Table S6: Root mean square errors (RMSEs) of each logistic parameter for the four-component bivariate model from 100 replicates of 250 four-component bivariate time series of length 50. RMSEs of the proposed method were compared to TRAJ procedure in SAS. Parameters  $\delta_0$ ,  $\delta_1$ ,  $\delta_2$  and  $\delta_3$  are intercept, first, second and third logistic parameters, respectively. The fourth component was used as the reference component. The true values of logistic parameters are 5,  $-3.5$ ,  $1$ ,  $0.1$  (first component),  $-4$ ,  $2.5$ ,  $-2$ ,  $-0.2$  (second component),  $3$ ,  $-2$ ,  $0.8$ ,  $0.2$  (third component). C1, C2, C3 and C4 denote first, second, third and fourth component, respectively.

| n  | N   | Method   | Comparison | $\delta_0$ | $\delta_1$ | $\delta_2$ | $\delta_3$ |
|----|-----|----------|------------|------------|------------|------------|------------|
| 50 | 250 | Proposed | C1 vs C4   | 0.63       | 0.41       | 0.26       | 0.29       |
|    |     |          | C2 vs C4   | 1.00       | 0.46       | 0.40       | 0.27       |
|    |     |          | C3 vs C4   | 0.63       | 0.33       | 0.23       | 0.24       |
|    |     | TRAJ     | C1 vs C4   | 0.91       | 0.56       | 0.30       | 0.28       |
|    |     |          | C2 vs C4   | 1.40       | 0.86       | 0.61       | 0.35       |
|    |     |          | C3 vs C4   | 2.24       | 1.40       | 0.85       | 0.27       |

Table S7: Mean (standard deviation) of the averaged root square error (ARSE), the averaged bias (A-bias) and the variance of bias (V-bias) of estimated trajectories for each component from 100 replicates of 250 four-component bivariate time series of length 70. Estimates of the proposed method were compared to R package gbmt and TRAJ procedure in SAS. C1, C2, C3 and C4 denote first, second, third and fourth component, respectively. Means were calculated by averaging over estimates of 100 replicates. Standard deviations are Monte Carlo standard deviations from estimates of 100 replicates. Each value was reported  $\times 10^2$ .

| n  | N   | Method   | ARSE C1 | A-bias C1 | V-bias C1 | ARSE C2 | A-bias C2 | V-bias C2 |
|----|-----|----------|---------|-----------|-----------|---------|-----------|-----------|
| 70 | 250 | Proposed | 2.94    | -0.04     | 0.08      | 2.61    | -0.01     | 0.06      |
|    |     |          | (0.60)  | (1.06)    | (0.04)    | (0.57)  | (0.87)    | (0.03)    |
|    |     | gbmt     | 3.10    | -0.04     | 0.09      | 3.18    | 0.01      | 0.10      |
|    |     |          | (0.63)  | (1.06)    | (0.04)    | (0.70)  | (1.05)    | (0.05)    |
|    |     | TRAJ     | 13.52   | -1.58     | 3.71      | 11.51   | -0.19     | 2.54      |
|    |     |          | (17.70) | (11.09)   | (8.80)    | (14.85) | (9.98)    | (7.10)    |
| n  | N   | Method   | ARSE C3 | A-bias C3 | V-bias C3 | ARSE C4 | A-bias C4 | V-bias C4 |
| 70 | 250 | Proposed | 3.30    | -0.02     | 0.10      | 2.85    | -0.07     | 0.08      |
|    |     |          | (0.76)  | (1.21)    | (0.05)    | (0.73)  | (0.97)    | (0.04)    |
|    |     | gbmt     | 3.51    | -0.01     | 0.12      | 3.26    | -0.09     | 0.10      |
|    |     |          | (0.79)  | (1.21)    | (0.06)    | (0.80)  | (1.06)    | (0.05)    |
|    |     | TRAJ     | 13.07   | 1.48      | 2.90      | 10.68   | 0.65      | 2.16      |
|    |     |          | (15.21) | (10.52)   | (7.11)    | (12.93) | (8.11)    | (5.66)    |

Table S8: Root mean square errors (RMSEs) of each logistic parameter for the four-component bivariate model from 100 replicates of 250 four-component bivariate time series of length 70. RMSEs of the proposed method were compared to TRAJ procedure in SAS. Parameters  $\delta_0$ ,  $\delta_1$ ,  $\delta_2$  and  $\delta_3$  are intercept, first, second and third logistic parameters, respectively. The fourth component was used as the reference component. The true values of logistic parameters are 5,  $-3.5$ , 1, 0.1 (first component),  $-4, 2.5, -2, -0.2$  (second component), 3,  $-2, 0.8, 0.2$  (third component). C1, C2, C3 and C4 denote first, second, third and fourth component, respectively.

| n  | N   | Method   | Comparison | $\delta_0$ | $\delta_1$ | $\delta_2$ | $\delta_3$ |
|----|-----|----------|------------|------------|------------|------------|------------|
| 70 | 250 | Proposed | C1 vs C4   | 0.64       | 0.40       | 0.26       | 0.28       |
|    |     |          | C2 vs C4   | 0.92       | 0.42       | 0.41       | 0.28       |
|    |     |          | C3 vs C4   | 0.63       | 0.31       | 0.23       | 0.23       |
|    |     | TRAJ     | C1 vs C4   | 0.82       | 0.50       | 0.27       | 0.28       |
|    |     |          | C2 vs C4   | 1.47       | 0.86       | 0.61       | 0.36       |
|    |     |          | C3 vs C4   | 1.60       | 0.96       | 0.57       | 0.25       |

## APPENDIX C: ADDITIONAL REAL-DATA RESULTS

Appendix C gives more real-data results in addition to real-data application in Section 7 of the paper. Our motivating study is given in Section 2 of the paper. Figure S1 shows estimated trajectories of the three-component model for another set of four channels (S1D3, S3D2, S5D4, and S7D4). Based on the selection criterion adjust DIC introduced in Section 5.2 of the paper, the three-component model was selected as the best model. We named the second component as the mixture response component because it involves both increased and decreased brain activity or hemoglobin level for the still-face period for different channels. In addition, Figure S2 gives logistic coefficient estimates and 95% credible intervals for each covariate for the previous model. Notably, the last component (third component) is always used as the reference component. We are able to reach the same conclusion with the positive estimates of IBQ negative scores and negative estimates of IBQ effortful scores for both components (component 1 vs 3, component 2 vs 3).

In addition to four-channel analyses, we also present results from all channels (twelve channels). Figures S3, S4, S5 are estimated trajectories of the first, second and third component for the three-component model with all twelve channels, respectively. The three-component model was selected as the best model for the twelve-channel analysis based on adjusted DIC. We named three components no response, mixture response, and response component, respectively. Figure S6 gives logistic coefficient estimates and 95 % credible intervals for each covariate of the previous model.

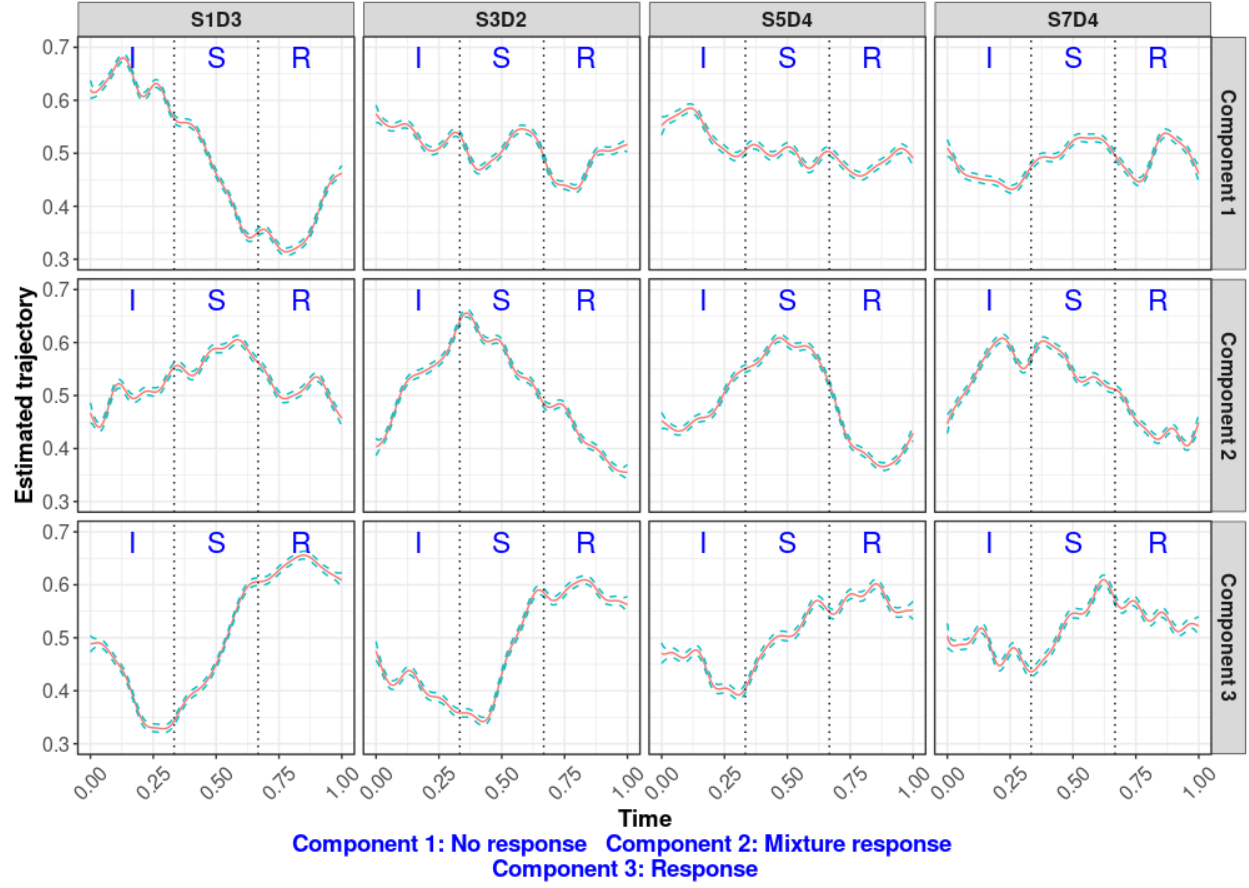

Figure S1: Estimated trajectories of the three-component model with four selected channels. **I**: Interact **S**: Still-face **R**: Recovery. Red curves are posterior mean and two green dashed curves are 95% pointwise credible intervals.

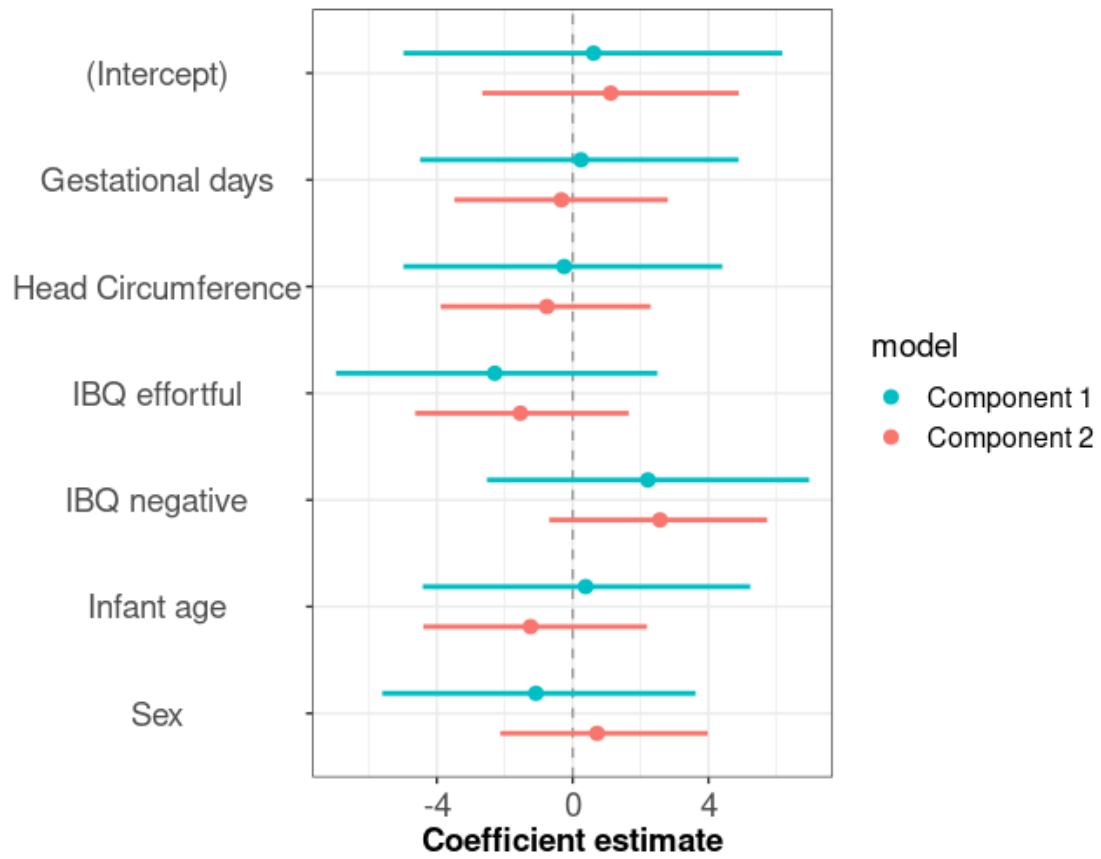

Figure S2: Logistic coefficient estimates and 95% credible intervals for each covariate of the three-component model.

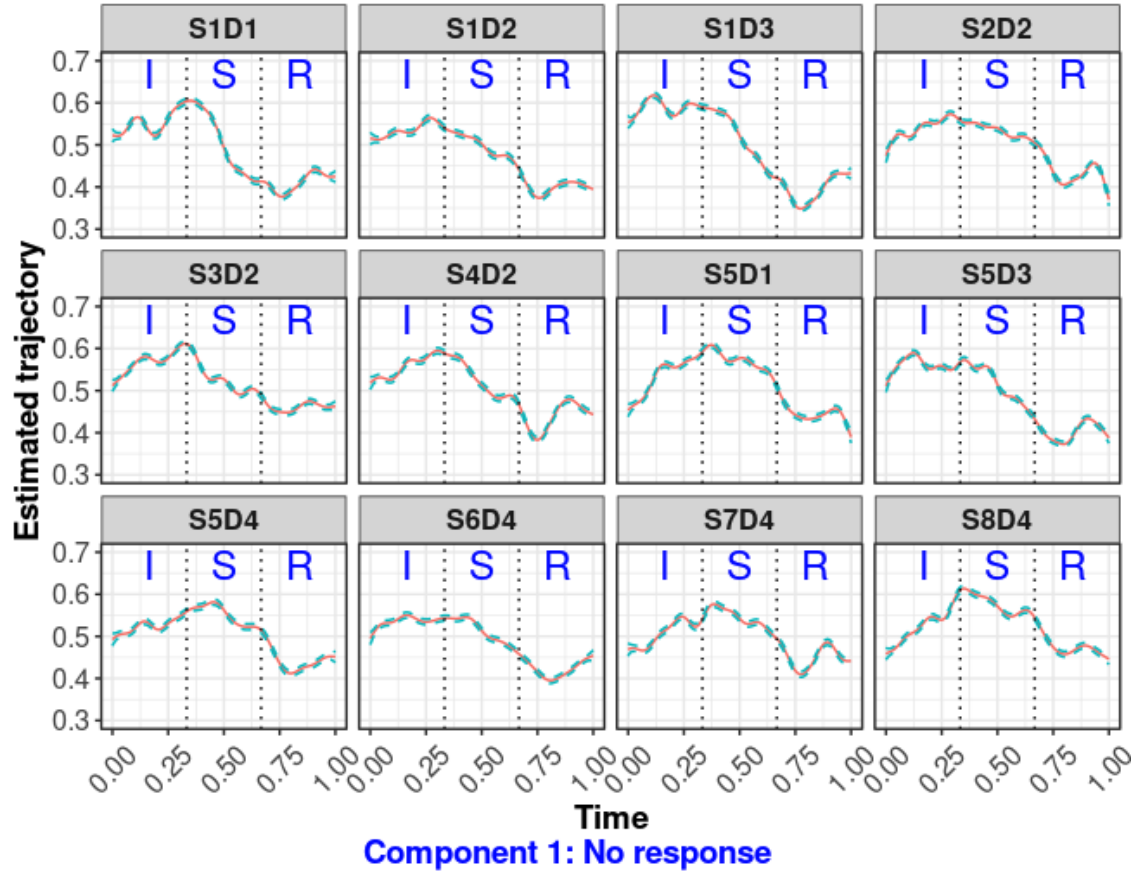

Figure S3: Estimated trajectories of the first component for the three-component model with all twelve channels. **I**: Interact **S**: Still-face **R**: Recovery. Red curves are posterior mean and two green dashed curves are 95% pointwise credible intervals.

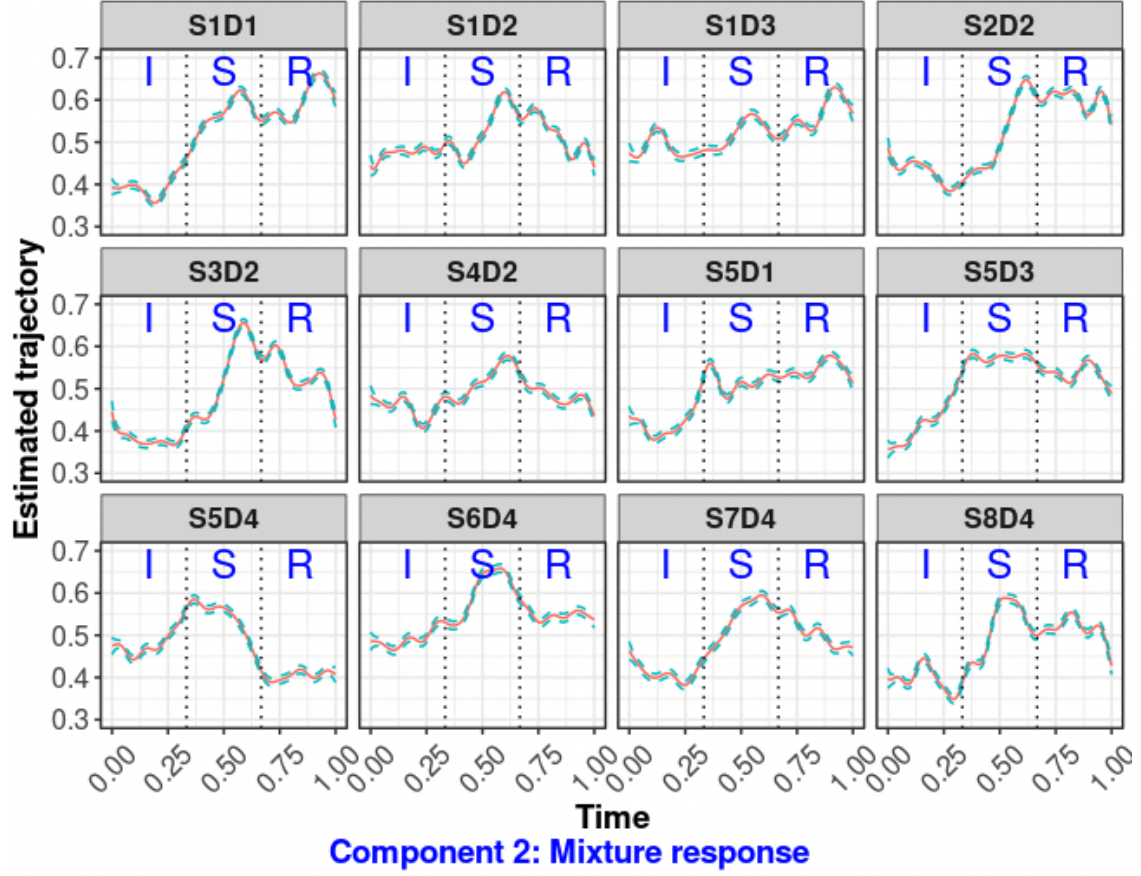

Figure S4: Estimated trajectories of the second component for the three-component model with all twelve channels. **I**: Interact **S**: Still-face **R**: Recovery. Red curves are posterior mean and two green dashed curves are 95% pointwise credible intervals.



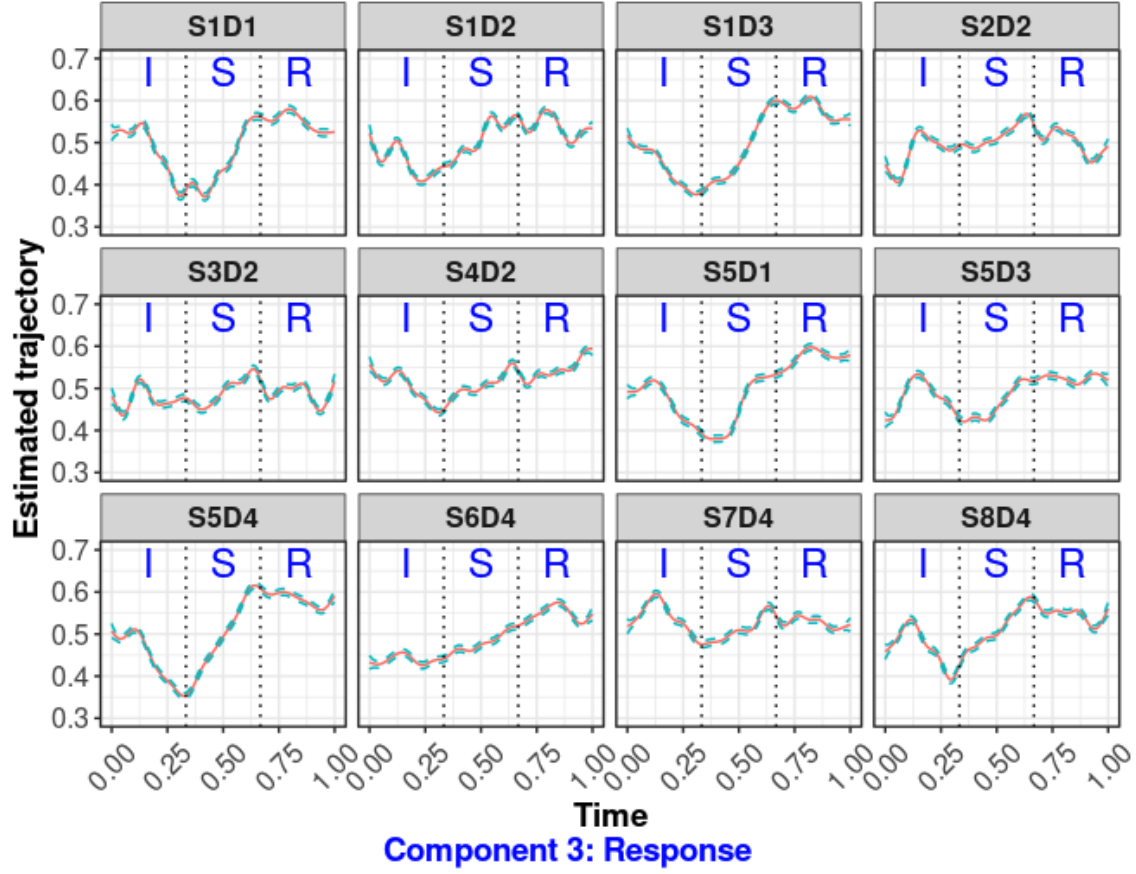

Figure S5: Estimated trajectories of the third component for the three-component model with all twelve channels. **I**: Interact **S**: Still-face **R**: Recovery. Red curves are posterior mean and two green dashed curves are 95% pointwise credible intervals.

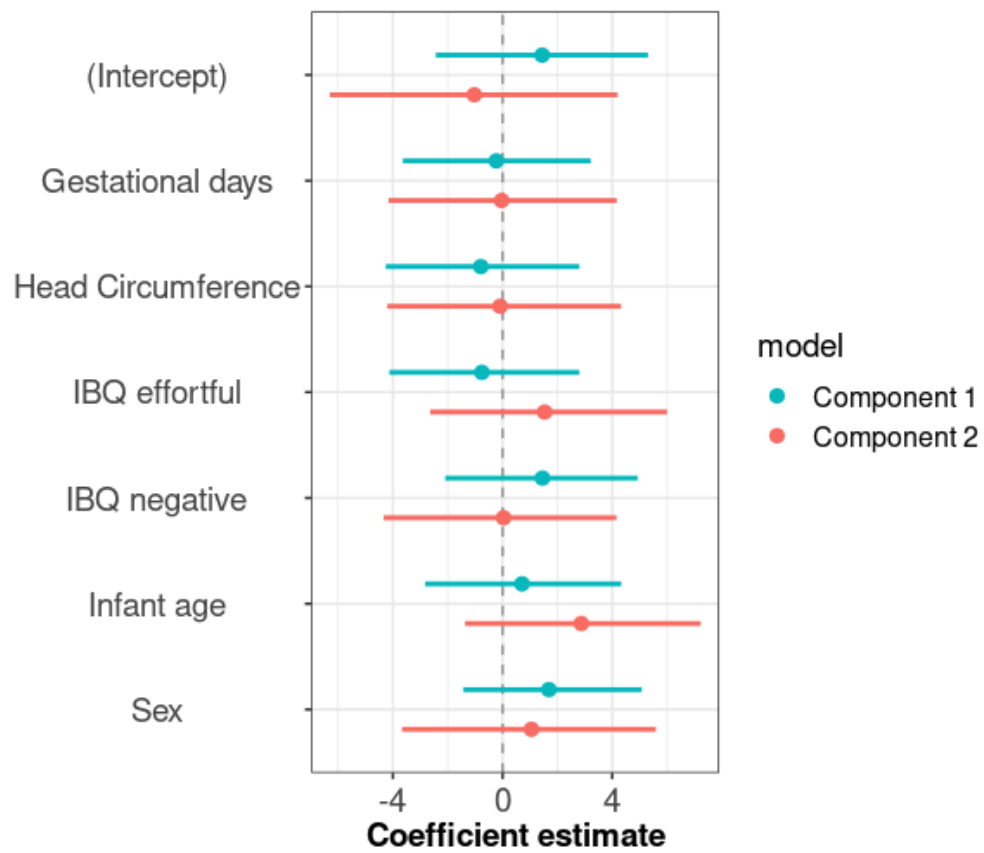

Figure S6: Logistic coefficient estimates and 95% credible intervals for each covariate of the three-component model for all twelve channels.

## References

- GELMAN, ANDREW. (2006). Prior distributions for variance parameters in hierarchical models (comment on article by browne and draper). *Bayesian analysis* **1**(3), 515–534.
- MAGRINI, ALESSANDRO. (2022). Assessment of agricultural sustainability in european union countries: a group-based multivariate trajectory approach. *AStA Advances in Statistical Analysis*, 1–31.
- NAGIN, DANIEL S, JONES, BOBBY L, PASSOS, VALERIA LIMA AND TREMBLAY, RICHARD E. (2018). Group-based multi-trajectory modeling. *Statistical methods in medical research* **27**(7), 2015–2023.
- POLSON, NICHOLAS G, SCOTT, JAMES G AND WINDLE, JESSE. (2013). Bayesian inference for logistic models using pólya–gamma latent variables. *Journal of the American statistical Association* **108**(504), 1339–1349.
- WAND, MATTHEW P, ORMEROD, JOHN T, PADOAN, SIMONE A AND FRÜHWIRTH, RUDOLF. (2011). Mean field variational bayes for elaborate distributions. *Bayesian Analysis* **6**(4), 847–900.
